# Supplementary material for: Semiclassical Approximations to Cosmological Perturbations
Source: arXiv:0705.3764 source file (2007-05-24)
Supplement: Supplementary file 1 [file appendice_WKB.tex]

\chapter{Approssimazione WKB e Sviluppo adiabatico}
\label{WKB_vs_adia}

In questa appendice daremo un senso all'equivalenza tra l'approccio WKB classico
e lo sviluppo adiabatico. In particolare tale prova sar\`{a} data per
l'ordine adiabatico $2$.

\section{Espansione WKB}

Questa sezione presenta l'approssimazione WKB cos\`{\i} come si trova su diversi testi
dedicati alla meccanica quantistica \cite{davydov,messiah,landau} o ai metodi matematici di risoluzione dei
problemi fisici \cite{bender_orszag}. Per rimanere aderenti al testo utilizzeremo, dove possibile,
le stesse notazioni, omettendo indici e pedici superflui.

L'equazione di nostro interesse \`{e} della forma

\begin{equation}
    \delta^{2}\,\frac{d^{2}\,u(x)}{dx^{2}}=Q(x)\,u(x)
    \label{schr_eq}
\end{equation}

\noindent con $Q(x)$ monotona crescente che passa da valori negativi a valori positivi.

La soluzione per $\delta\rightarrow 0$ si pu\`{o} scrivere come

\begin{equation}
    u(x)=\exp{\left[\frac{1}{\delta}\,\sum_{n=0}^{\infty}\delta^{n}\,S_{n}(x)\right]}\;.
    \label{WKB_sol_app}
\end{equation}

\noindent Questa \`{e} la formula di partenza dalla quale si deriva l'approssimazione WKB
ad un determinato ordine.

Ponendo (\ref{WKB_sol_app}) in (\ref{schr_eq}) e troncando la serie ad un numero finito
di termini $L$, troviamo, eguagliando i termini nelle potenze di $\delta$,
 un sistema di equazioni differenziali nelle derivate di $S_{l}(x)$ con
$l$ compreso tra $0$ e $L$. Risolvendo tale sistema di equazioni differenziali determiniamo
le $S_{l}(x)$ di nostro interesse come funzioni delle derivate di $Q(x)$. I primi termini dello
sviluppo in (\ref{WKB_sol_app}) sono

\begin{equation}
    S_{0}(x)=\pm\,\int^{x}\sqrt{Q(t)}\,dt
    \label{S0_x}
\end{equation}

\noindent soluzione della cosidetta \emph{equazione eikonale}: $S_{0}'^{2}=Q(x)$
\footnote{Da qui l'apice indicher\`{a} la derivazione nella variabile considerata per $S_{j}$ e $Q$.}

\begin{equation}
    S_{1}(x)=-\,\frac{1}{4}\,\ln Q(x)
    \label{S1_x}
\end{equation}

\noindent soluzione della cosidetta \emph{equazione di trasporto}:
$2\,S_{0}'\,S_{1}'\,+\,S_{0}''=0$

\begin{equation}
    S_{2}(x)=\pm\,\int^{x}\left[\frac{Q''}{8\,Q^{3/2}}-\frac{5\,(Q')^{2}}{32\,Q^{5/2}}\right]\,dt
    \label{S2_x}
\end{equation}

\noindent e

\begin{equation}
    S_{3}(x)=-\frac{Q''}{16\,Q^{2}}+\frac{5\,(Q')^{2}}{64\,Q^{3}}\;.
    \label{S3_x}
\end{equation}

Scriviamo ora la soluzione al quart'ordine WKB (con $S_{0},S_{1},S_{2},S_{3}$)
raccogliendo i fattori comuni\footnote{In questa appendice l'ordine a cui ci si
riferisce per l'approssimazione WKB \`{e} da intendersi come il numero di termini $S_{j}$
che si considerano, partendo da $S_{0}$.}

\begin{equation}
    \begin{array}{ll}
    u^{(4)}_{wkb}(x)=e^{-\frac{1}{4}\,\ln Q(x)}\,
    \left\{A_{+}\,e^{\left[\frac{1}{\delta}\,\left(\int^{x}\sqrt{Q(t)}\,dt
    +\delta^{2}\,\int^{x}\left[\frac{Q''}{8\,Q^{3/2}}-\frac{5\,Q'^{2}}{32\,Q^{5/2}}\right]dt\right)\right]}
    \right.\\
    \\
    \left.\quad+A_{-}\,e^{\left[\frac{1}{\delta}\,\left(
    -\int^{x}\sqrt{Q(t)}\,dt
    -\delta^{2}\,\int^{x}\left[\frac{Q''}{8\,Q^{3/2}}-\frac{5\,Q'^{2}}{32\,Q^{5/2}}\right]dt\right)\right]}
    \right\}\,
    e^{\delta^{2}\,\left(-\frac{Q''}{16\,Q^{2}}+\frac{5\,Q'^{2}}{64\,Q^{3}}\right)}
    \end{array}
    \label{sol_WKB_4_racc}
\end{equation}

\noindent ora, con $\delta=1$ e semplificando ulteriormente

\begin{equation}
    \begin{array}{ll}
    u^{(4)}_{wkb}(x)=\frac{1}{\left[Q(x)\right]^{1/4}}\,
    \left\{A_{+}\,e^{\left[\int^{x}\left(\sqrt{Q(t)}\,
    +\frac{Q''}{8\,Q^{3/2}}-\frac{5\,Q'^{2}}{32\,Q^{5/2}}\right)dt\right]}
    \right.\\
    \\
    \left.\qquad\qquad\qquad+A_{-}\,e^{\left[-\,\int^{x}\left(\sqrt{Q(t)}\,
    +\frac{Q''}{8\,Q^{3/2}}-\frac{5\,Q'^{2}}{32\,Q^{5/2}}\right)dt\right]}
    \right\}\,
    e^{\left(-\frac{Q''}{16\,Q^{2}}+\frac{5\,Q'^{2}}{64\,Q^{3}}\right)}\;.
    \end{array}
    \label{sol_WKB_4_semp}
\end{equation}

\section{Sviluppo adiabatico}

Questa sezione presenta la tecnica dello sviluppo adiabatico al second'ordine come viene
presentata da Birrell e Davies in \cite{birrel}. La notazione che utiliziamo \`{e} quella del capitolo
\ref{WKB} omettendo le scritture non essenziali.

Come gi\`{a} indicato la soluzione formale all'ordine adiabatico $2$
\`{e} \footnote{Tralasciando la normalizzazione, inutile per lo scopo dell'appendice, ed indicando
anche la soluzione con il segno $+$ nell'esponenziale.}

\begin{equation}
    u^{(2)}(x)=\frac{1}{\sqrt{W^{(2)}(x)}}\,\left\{
    \widetilde{A}_{+}\,e^{\left[i\,\int^{x}W^{(2)}(t)\, dt\right]}
    +\widetilde{A}_{-}\,e^{\left[-\,i\,\int^{x}W^{(2)}(t)\, dt\right]}
    \right\}
    \label{WKB_formal_sol_2_app}
\end{equation}

\noindent con

\begin{equation}
    W^{(2)}(x)=\omega(x)\,\left[1+\sigma_{2}(x)\right]^{\frac{1}{2}}
    \label{W_2th_order_app}
\end{equation}

\noindent e

\begin{equation}
    \sigma_{2}=-\,\frac{1}{2}\,\frac{\ddot{\omega}}{\omega^{3}}
    +\frac{3}{4}\,\frac{\dot{\omega}^{2}}{\omega^{4}}\;.
    \label{sigma2j_app}
\end{equation}

Esplicitando in parte la scritura (\ref{WKB_formal_sol_2_app}) abbiamo

\begin{equation}
\begin{array}{ll}
    u^{(2)}(x)=\frac{1}{\sqrt{\omega(x)\,\left[1+\sigma_{2}(x)\right]^{\frac{1}{2}}}}\,\left\{
    \widetilde{A}_{+}\,e^{\left[i\,\int^{x}\omega(t)\,\left[1+\sigma_{2}(t)\right]^{\frac{1}{2}}\, dt\right]}
    \right.\\
    \\
    \left.\qquad\qquad\qquad\qquad\qquad\qquad+
    \widetilde{A}_{-}\,e^{\left[-\,i\,\int^{x}\omega(t)\,\left[1+\sigma_{2}(t)\right]^{\frac{1}{2}}\, dt\right]}
    \right\}\;.
\end{array}
    \label{WKB_formal_sol_2_app_esplic}
\end{equation}

Occorre ora dimostrare che le due formule (\ref{sol_WKB_4_semp}) e (\ref{WKB_formal_sol_2_app_esplic})
sono equivalenti ed in quali approssimazioni.

\section{Relazioni tra $Q(x)$ e $\omega(x)$}

Cominciamo con l'esprimere le funzioni di $Q(x)$ e delle sue derivate nella (\ref{sol_WKB_4_semp})
come funzioni di $\omega(x)$ e delle sue derivate. Sapendo che la nostra equazione \`{e}
\begin{equation}
    \frac{d^{2}u(x)}{dx^{2}}+\omega^{2}(x)\,u(x)=0
    \label{eq_moto_u_with_x_app}
\end{equation}

\noindent la riscriviamo nella forma di (\ref{schr_eq})

\begin{equation}
    \frac{d^{2}\,u(x)}{dx^{2}}=-\omega^{2}(x)\,u(x)
    \label{schr_eq_for_us}
\end{equation}

\noindent con $-\omega^{2}(x)$ anch'essa monotona crescente che passa da valori negativi
a valori positivi. Abbiamo quindi l'identificazione

\begin{equation}
    Q(x)=-\omega^{2}(x)\;.
    \label{identif}
\end{equation}

Possiamo identificare i termini che compaiono in (\ref{sol_WKB_4_semp})
\footnote{Qui gli apici ed i punti indicano sempre la derivazione in $x$ ma si preferisce adottarli
diversi rispettivamente per le derivate di $Q(x)$ e per le derivate di $\omega(x)$.}

\begin{equation}
    \sqrt{Q(x)}=i\,\omega(x)\;,
    \label{1st_id}
\end{equation}

\begin{equation}
    \frac{Q''}{8\,Q^{3/2}}-\frac{5\,Q'^{2}}{32\,Q^{5/2}}=i
    \left(\frac{3}{8}\,\frac{\dot{\omega}^{2}}{\omega^{3}}
    -\,\frac{1}{4}\,\frac{\ddot{\omega}}{\omega^{2}}\right)\;,
    \label{2nd_id}
\end{equation}

\begin{equation}
    -\frac{Q''}{16\,Q^{2}}+\frac{5\,Q'^{2}}{64\,Q^{3}}=
    \frac{1}{8}\,\frac{\ddot{\omega}}{\omega^{3}}
    -\,\frac{3}{16}\,\frac{\dot{\omega}^{2}}{\omega^{4}}\;.
    \label{3th_id}
\end{equation}

\section{Confronto}

Scriviamo ora la (\ref{sol_WKB_4_semp}) con $\omega(x)$ e la sue derivate

\begin{equation}
    \begin{array}{ll}
    u^{(4)}_{wkb}(x)=\frac{1}{\sqrt{i}\,\sqrt{\omega(x)}}\,
    \left\{A_{+}\,e^{\left[i\,\int^{x}\left(\omega(t)\,
    +\frac{3}{8}\,\frac{\dot{\omega}^{2}}{\omega^{3}}
    -\,\frac{1}{4}\,\frac{\ddot{\omega}}{\omega^{2}}\right)dt\right]}
    \right.\\
    \\
    \left.\qquad\qquad\qquad+A_{-}\,e^{\left[-\,i\,\int^{x}\left(\omega(t)\,
    +\frac{3}{8}\,\frac{\dot{\omega}^{2}}{\omega^{3}}
    -\,\frac{1}{4}\,\frac{\ddot{\omega}}{\omega^{2}}\right)dt\right]}
    \right\}\,
    e^{\left(\frac{1}{8}\,\frac{\ddot{\omega}}{\omega^{3}}
    -\,\frac{3}{16}\,\frac{\dot{\omega}^{2}}{\omega^{4}}\right)}
    \end{array}
    \label{sol_WKB_4_with_om}
\end{equation}

\noindent dove la radice di $i$ sar\`{a} riassorbita nella redefinizione della costanti $A_{\pm}$
che diventano $\widetilde{A}_{\pm}$.

Determiniamo quali altre approssimazioni occorrono per arrivare ad una completa identificazione tra (\ref{sol_WKB_4_with_om}) e (\ref{WKB_formal_sol_2_app_esplic}). Cominciamo con lo sviluppare
l'argomento dell'integrale in (\ref{WKB_formal_sol_2_app_esplic}) per piccoli $\sigma_{2}$
\footnote{Questo \`{e} lecito nel regime adiabatico.}

\begin{equation}
    W^{(2)}(x)=\omega(x)\,\left[1+\sigma_{2}(x)\right]^{\frac{1}{2}}
    \cong\omega(x)\,\left(1+\frac{1}{2}\,\sigma_{2}(x)\right)
    \label{W_2th_order_app_svil}
\end{equation}

\noindent ed anche

\begin{equation}
    \frac{1}{\sqrt{W^{(2)}(x)}}=\frac{1}{\sqrt{\omega(x)\,\left[1+\sigma_{2}(x)\right]^{\frac{1}{2}}}}
    \cong\frac{1}{\sqrt{\omega(x)}}\,\left(1-\frac{1}{4}\,\sigma_{2}(x)\right)\;.
    \label{W_2th_order_app_svil_freq}
\end{equation}

Sostituendo $\sigma_{2}$ abbiamo l'argomento dell'esponenziale

\begin{equation}
    W^{(2)}(x)
    \cong\omega(x)\,\left[1+\frac{1}{2}\,\left(-\,\frac{1}{2}\,\frac{\ddot{\omega}}{\omega^{3}}
    +\frac{3}{4}\,\frac{\dot{\omega}^{2}}{\omega^{4}}\right)\right]
    =\omega(x)-\,\frac{1}{4}\,\frac{\ddot{\omega}}{\omega^{2}}
    +\frac{3}{8}\,\frac{\dot{\omega}^{2}}{\omega^{3}}
    \label{W_2th_order_app_svil_sost}
\end{equation}

\noindent e

\begin{equation}
    \frac{1}{\sqrt{W^{(2)}(x)}}
    \cong\frac{1}{\sqrt{\omega(x)}}\,\left[1+\left(\frac{1}{8}\,\frac{\ddot{\omega}}{\omega^{3}}
    -\frac{3}{16}\,\frac{\dot{\omega}^{2}}{\omega^{4}}\right)\right]\;.
    \label{W_2th_order_app_svil_freq_sost}
\end{equation}

Riscriviamo la (\ref{WKB_formal_sol_2_app}) con quanto appena trovato

\begin{equation}
\begin{array}{ll}
    u^{(2)}(x)=\frac{\left[1+\left(\frac{1}{8}\,\frac{\ddot{\omega}}{\omega^{3}}
    -\frac{3}{16}\,\frac{\dot{\omega}^{2}}{\omega^{4}}\right)\right]}{\sqrt{\omega(x)}}\,\left\{
    \widetilde{A}_{+}\,e^{\left[i\,\int^{x}\left(\omega(t)-\,\frac{1}{4}\,\frac{\ddot{\omega}}{\omega^{2}}
    +\frac{3}{8}\,\frac{\dot{\omega}^{2}}{\omega^{3}}\right)\, dt\right]}\right.\\
    \\
    \left.\qquad\qquad\qquad\qquad\qquad
    +\widetilde{A}_{-}\,e^{\left[-\,i\,\int^{x}\left(\omega(t)-\,\frac{1}{4}\,\frac{\ddot{\omega}}{\omega^{2}}
    +\frac{3}{8}\,\frac{\dot{\omega}^{2}}{\omega^{3}}\right)\, dt\right]}
    \right\}\;.
\end{array}
    \label{WKB_formal_sol_2_app_sost}
\end{equation}

Ora per passare da $u^{(4)}_{wkb}$ a $u^{(2)}$ occorre sviluppare l'esponenziale che compare
nella soluzione WKB

\begin{equation}
    e^{\left(\frac{1}{8}\,\frac{\ddot{\omega}}{\omega^{3}}
    -\,\frac{3}{16}\,\frac{\dot{\omega}^{2}}{\omega^{4}}\right)}
    \cong1+\left(\frac{1}{8}\,\frac{\ddot{\omega}}{\omega^{3}}
    -\frac{3}{16}\,\frac{\dot{\omega}^{2}}{\omega^{4}}\right)\;.
    \label{svil_exp}
\end{equation}

Abbiamo mostrato che l'approssimazione WKB al quart'ordine e lo sviluppo adiabatico
al secondo coincidono a meno di termini di ordine superiore.

L'ordine adiabatico $0$ coincide con l'approssimazione WKB all'ordine $2$
(con $S_{0},S_{1}$ - approssimazione dell'ottica fisica),
come si vede immediatamente osservando le formule (\ref{sol_WKB_4_with_om}) e
(\ref{WKB_formal_sol_2_app_sost}) e tralasciando i termini in $\dot{\omega}$ e in
$\ddot{\omega}$ (ovvero senza considerare le correzioni $S_{2},S_{3}$ per la WKB
e $\sigma_{2}$ per lo sviluppo adiabatico).

\vspace{30cm}

$\phantom{\mu}$
